# Supplementary material for: Kelvin-Helmholtz instability of the Dirac fluid of charge carriers on graphene
Source: arXiv:1706.00801 source file (2017-11-28)
Supplement: Supplementary file 1 [file SM.pdf]

# Supplemental Material: Kelvin-Helmholtz instability on the Dirac fluid of charge carriers in graphene

Rodrigo C. V. Coelho,[1,2,*] Miller Mendoza,[2,†] Mauro M. Doria,[1,‡] and Hans J. Herrmann[2,§]

[1]*Departamento de Física dos Sólidos, Universidade Federal do Rio de Janeiro, 21941-972 Rio de Janeiro, Brazil*
[2]*ETH Zürich, Computational Physics for Engineering Materials, Institute for Building Materials Schafmattstrasse 6, HIF, CH-8093 Zürich, Switzerland*

(Dated: November 14, 2017)

The aim of this Supplemental Material is to give more details about the model we use to simulate the Kelvin-Helmholtz instability on graphene. We show in three sections the relativistic polynomials up to fifth order as well as their coefficients, the gaussian quadrature with high precision and the full expansion of the Fermi-Dirac expansion up to fifth order. A relativistic lattice Boltzmann method (LBM)[1, 2] is used to simulate the fluid flow, which is a numerical method to solve the relativistic Boltzmann equation,

$$\bar{p}^\mu \partial_\mu f = -\frac{\bar{p}_\mu U^\mu}{v_F^2 \tau}(f - f^{eq}), \tag{0.1}$$

where $v_F$ is the Fermi speed and $\tau$ is the relaxation time. We assume here the Einstein's notation, where repeated indexes represent a sum. The greek indexes range from 0 to 2 while the latin ones range from 1 to 2. The relativistic momentum is denoted by $\bar{p}^\mu = (E/v_F, \bar{\mathbf{p}})$, the velocity is $U^\mu = \gamma(v_F, \mathbf{u})$ and the time-space coordinates are $x^\mu = (v_F t, \mathbf{x})$, where $\gamma(u) = 1/\sqrt{1 - u^2/v_F^2}$ is the Lorentz factor. The ultrarelativistic limit, i.e, the kinetic energy is much greater than the rest mass energy, is considered, since the electrons in graphene behave effectively as a Dirac fluid of massless quasi-particles moving with the Fermi speed[3], which implies $\bar{p}^\mu \bar{p}_\mu = (\bar{p}^0)^2 - \bar{\mathbf{p}}^2 = 0 \;\Rightarrow\; \bar{p}^0 = |\bar{\mathbf{p}}|$. We also use natural units: $v_F = k_B = \hbar = e = 1$.

## I. POLYNOMIALS

In LBM, the equilibrium distribution function (EDF), which is the Fermi-Dirac distribution in our model, is expanded in orthogonal polynomials so as the gaussian quadrature gives exact results for the integrations. For our problem, we develop relativistic polynomials by the a Gram-Schmidt procedure, with the following orthogonalization:

$$\int \frac{d^2p}{p^0}\omega(p) P^{i_1\cdots i_N} P^{j_1\cdots j_M} = \delta_{NM}\delta^{i_1\cdots i_N|j_1\cdots j_N}, \tag{1.1a}$$

$$\int \frac{d^2p}{p^0}\omega(p) P^{i_1\cdots i_N 0} P^{j_1\cdots j_M 0} = \delta_{NM}\delta^{i_1\cdots i_N|j_1\cdots j_N}, \tag{1.1b}$$

$$\int \frac{d^2p}{p^0}\omega(p) P^{i_1\cdots i_N 0} P^{j_1\cdots j_M} = 0. \tag{1.1c}$$

where $\omega(p)$ is the weight function, which for graphene with zero chemical potential reads:

$$\omega(p) = \frac{1}{e^p + 1}. \tag{1.2}$$

Here the normalization factor is the same as for the Hermite polynomials in D-dimensions[4–6], where we define $\delta_{i_1\cdots i_N|j_1\cdots j_N} \equiv \delta_{i_1 j_1}\cdots\delta_{i_N j_N}$ + all permutations of $j$'s and $\delta^{ij}$ is the Kronecker's delta. See below the general form of the polynomials up to fifth order:

$$P = A_1, \quad P^{i_1} = B_1 p^{i_1}, \quad P^0 = C_1 p + C_2, \quad P^{i_1 i_2} = D_1 p^{i_1} p^{i_2} + (D_2 p^2 + D_3 p + D_4)\delta^{i_1 i_2} \tag{1.3}$$

* rcvcoelho@if.ufrj.br
† mmendoza@ethz.ch
‡ mmd@if.ufrj.br
§ hans@ifb.baug.ethz.ch

$$P^{i_1 0} = (E_1 p + E_2) p^{i_1}, \quad P^{i_1 i_2 i_3} = F_1 p^{i_1} p^{i_2} p^{i_3} + (F_2 p^2 + F_3 p + F_4)(p^{i_1}\delta^{i_2 i_3} + p^{i_2}\delta^{i_1 i_3} + p^{i_3}\delta^{i_1 i_2}) \tag{1.4}$$

$$P^{i_1 i_2 0} = (G_1 p + G_2) p^{i_1} p^{i_2} + \delta^{i_1 i_2}(G_3 p^3 + G_4 p^2 + G_5 p + G_6) \tag{1.5}$$

$$P^{i_1 i_2 i_3 i_4} = H_1 p^{i_1} p^{i_2} p^{i_3} p^{i_4} + (H_2 p^2 + H_3 p + H_4)(p^{i_1} p^{i_2}\delta^{i_3 i_4} + p^{i_1} p^{i_3}\delta^{i_2 i_4} + p^{i_1} p^{i_4}\delta^{i_2 i_3} + p^{i_2} p^{i_3}\delta^{i_1 i_4} + p^{i_2} p^{i_4}\delta^{i_1 i_3} + p^{i_3} p^{i_4}\delta^{i_1 i_2}) + (H_5 p^4 + H_6 p^3 + H_7 p^2 + H_8 p + H_9)\delta^{i_1 i_2 i_3 i_4} \tag{1.6}$$

$$P^{i_1 i_2 i_3 0} = (I_1 p + I_2) p^{i_1} p^{i_2} p^{i_3} + (I_3 p^3 + I_4 p^2 + I_5 p + I_6)(p^{i_1}\delta^{i_2 i_3} + p^{i_2}\delta^{i_1 i_3} + p^{i_3}\delta^{i_1 i_2}) \tag{1.7}$$

$$P^{i_1 i_2 i_3 i_4 i_5} = J_1 p^{i_1} p^{i_2} p^{i_3} p^{i_4} p^{i_5} + (J_2 p^2 + J_3 p + J_4)(p^{i_3} p^{i_4} p^{i_5}\delta^{i_1 i_2} + p^{i_2} p^{i_4} p^{i_5}\delta^{i_1 i_3} + p^{i_2} p^{i_3} p^{i_5}\delta^{i_1 i_4} + p^{i_2} p^{i_3} p^{i_4}\delta^{i_1 i_5} + p^{i_1} p^{i_4} p^{i_5}\delta^{i_2 i_3} + p^{i_1} p^{i_3} p^{i_5}\delta^{i_2 i_4} + p^{i_1} p^{i_3} p^{i_4}\delta^{i_2 i_5} + p^{i_1} p^{i_2} p^{i_5}\delta^{i_3 i_4} + p^{i_1} p^{i_2} p^{i_4}\delta^{i_3 i_5} + p^{i_1} p^{i_2} p^{i_3}\delta^{i_4 i_5}) + (J_5 p^4 + J_6 p^3 + J_7 p^2 + J_8 p + J_9)(p^{i_1}\delta^{i_2 i_3 i_4 i_5} + p^{i_2}\delta^{i_1 i_3 i_4 i_5} + p^{i_3}\delta^{i_1 i_2 i_4 i_5} + p^{i_4}\delta^{i_1 i_2 i_3 i_5} + p^{i_5}\delta^{i_1 i_2 i_3 i_4}) \tag{1.8}$$

$$P^{i_1 i_2 i_3 i_4 0} = (K_1 p + K_2) p^{i_1} p^{i_2} p^{i_3} p^{i_4} + (K_3 p^3 + K_4 p^2 + K_5 p + K_6)(p^{i_3} p^{i_4}\delta^{i_1 i_2} + p^{i_2} p^{i_4}\delta^{i_1 i_3} + p^{i_2} p^{i_3}\delta^{i_1 i_4} + p^{i_1} p^{i_4}\delta^{i_2 i_3} + p^{i_1} p^{i_3}\delta^{i_2 i_4} + p^{i_1} p^{i_2}\delta^{i_3 i_4}) + (K_7 p^5 + K_8 p^4 + K_9 p^3 + K_{10} p^2 + K_{11} p + K_{12})\delta^{i_1 i_2 i_3 i_4} \tag{1.9}$$

After applying Eqs.(1.1) with the weight function in Eq.(1.2), we find the following coefficients for the polynomials:

| Coefficients for the polynomials | | | |
|---|---|---|---|
| $A_1$ | 0.479178512802528099359 | $B_1$ | 0.420162144163116575919 |
| $C_1$ | -0.438644124462952026498 | $C_2$ | 0.520481568553045876911 |
| $D_1$ | -0.233608989389108006407 | $D_2$ | -0.097441004413398425703 |
| $D_3$ | 0.917597045579769802408 | $D_4$ | -0.531475000588975578840 |
| $E_1$ | -0.2422247573630216072834 | $E_2$ | 0.763412795154197003902 |
| $F_1$ | -0.103390027980148910695 | $F_2$ | -0.034487194253661956789 |
| $F_3$ | 0.497679176861580881375 | $F_4$ | -0.787677504156166562193 |
| $G_1$ | -0.105145692979121715529 | $G_2$ | 0.532992207396207113467 |
| $G_3$ | -0.018002883696682218035 | $G_4$ | 0.393750481276605935516 |
| $G_5$ | -1.412420536798268410807 | $G_6$ | 0.536990688435255488358 |
| $H_1$ | -0.038969930308370242115 | $H_2$ | -0.011080524390703751100 |
| $H_3$ | 0.213394348146601288690 | $H_4$ | -0.543343339611386537125 |
| $H_5$ | -0.001561775510992725660 | $H_6$ | 0.074095215773109831851 |
| $H_7$ | -0.802501886208720176718 | $H_8$ | 1.916560801015023818452 |
| $H_9$ | -0.540434081091062445460 | $I_1$ | -0.039217041702671633262 |
| $I_2$ | 0.275525771736009317417 | $I_3$ | -0.005720483825062511177 |
| $I_4$ | 0.169014628075014851651 | $I_5$ | -0.983557036184103758269 |
| $I_6$ | 1.039602964347412266588 | $J_1$ | -0.012980727644304316166 |
| $J_2$ | -0.003293121530373324716 | $J_3$ | 0.078969365409892639233 |
| $J_4$ | -0.278006887135326353965 | $J_5$ | -0.000392510072743078929 |
| $J_6$ | 0.023430514884233595564 | $J_7$ | -0.343764130645662945885 |
| $J_8$ | 1.332632547448642249020 | $J_9$ | -1.056984063842437016982 |
| $K_1$ | -0.013008192610242189999 | $K_2$ | 0.117184604048740181739 |
| $K_3$ | -0.001672210511396452841 | $K_4$ | 0.061915830095755708422 |
| $K_5$ | -0.495675381489720021628 | $K_6$ | 0.844215355098998003249 |
| $K_7$ | -0.000186298805996007738 | $K_8$ | 0.012179616524288047656 |
| $K_9$ | -0.233313830639162821450 | $K_{10}$ | 1.431765270179315000143 |
| $K_{11}$ | -2.427035803258861132046 | $K_{12}$ | 0.542840276987905644691 |

The coefficients above were found specifically for two dimensions (see Eqs.(1.1)) and for the weight function in Eq.(1.2) but is could straightforwardly be generalized for three dimensions and for other weight functions, since the polynomials are given in a tensorial form with generic coefficients.

## II. QUADRATURE

The gaussian quadrature is a numerical method to calculate integrals by converting then into sums. In our model, the integrals appears when we calculate the moments of order M,

$$T^{\mu_1\cdots\mu_M} = \int \frac{d^2p}{p^0} f^{eq} p^{\mu_1} \ldots p^{\mu_M} = \sum_{i=1}^{Q} f_i^{eq} p_i^{\mu_1} \ldots p_i^{\mu_M},$$

for instance, the energy momentum tensor (order 2) $T^{\mu\nu} = \int \frac{d^2p}{p^0} f^{eq} p^\mu p^\nu$, in order to extract from them the macroscopic fields, as the velocity and temperature, by using the Landau-Lifshiz decomposition[7].

To calculate the quadrature, we apply the quadrature equations,

$$\int \frac{d^2p}{p^0} \omega(p) p^{\mu_1} p^{\mu_2} \ldots p^{\mu_N} = \sum_{i=1}^{Q} w_i p_i^{\mu_1}, p_i^{\mu_2} \ldots p_i^{\mu_N}, \tag{2.1}$$

with $N$ ranging from 0 to 10 for all combinations of indexes, which range from 0 to 2. The weight functions is the same as the one used for the polynomials, Eq.(1.2). The quadrature we use has 12 unitary velocity vectors of modulus $v_F$, $\mathbf{v_i} = \mathbf{p_i}/|\mathbf{p_i}|$, equally distributed in the angular space, $\phi_i = i\pi/6$ for $i = 0, 1, \ldots, 11$, and 72 momentum vectors (6 for each velocity vector). See below the norms of the momentum vectors and the discrete weights.

| D2V72 lattice for FD | | | |
|---|---|---|---|
| $p_1$ | 0.25201744581969162719 | $w_1$ | 0.14654307542929734102 |
| $p_2$ | 1.28431414936632151066 | $w_2$ | 0.16065812528060654507 |
| $p_3$ | 3.10299817105989769440 | $w_3$ | 0.05069990622400731106 |
| $p_4$ | 5.87378987120738934512 | $w_4$ | 0.00490494311508280217 |
| $p_5$ | 9.92960529659646770256 | $w_5$ | 0.00012453490742404226 |
| $p_6$ | 16.07238534570181554016 | $w_6$ | $4.30094182313495021986 \times 10^{-7}$ |

The same procedure and velocity vectors could also be used for other weight functions.

## III. EXPANSION

In this section, we expand the Fermi-Dirac distribution up to fifth order in relativistic polynomials. To do so, we introduce some non-dimensional variables: $\theta = T/T_0$, $\mathbf{p} = \bar{\mathbf{p}}/T_0$ and $\mu = \bar{\mu}/T_0$, where $T_0$ is the initial temperature, and the Fermi-Dirac distribution becomes:

$$f_{FD}^{eq} = \frac{1}{z^{-1} \exp\left[p^0 \gamma (1 - \mathbf{v} \cdot \mathbf{u})/\theta\right] + 1}, \tag{3.1}$$

where $z = e^{\frac{\mu}{\theta}}$ is the fugacity. The expansion up to fifth order is given by:

$$f^{eq} = \frac{n}{2\pi g_2(z) \theta^2} \omega(\xi) \left[ \sum_{N=0}^{5} \frac{1}{N!} A^{i_1 \ldots i_N} P^{i_1 \ldots i_N} + \sum_{M=0}^{4} \frac{1}{M!} A^{i_1 \ldots i_M 0} P^{i_1 \ldots i_M 0} \right], \tag{3.2}$$

where Fermi-Dirac integral is

$$g_\nu(z) = \frac{1}{\Gamma(\nu)} \int_0^\infty \frac{x^{\nu-1}\, dx}{z^{-1} e^x \pm 1}, \tag{3.3}$$

and the projections of the EDF on the polynomials are

$$A^{\mu_1 \mu_2 \cdots \mu_N} = \int \frac{d^2\mathbf{p}}{p^0} f^{eq} P^{\mu_1 \mu_2 \cdots \mu_N}. \tag{3.4}$$

Note that we divide the density $n$ by a normalization factor $2\pi\theta^2 g_2(z)$, since $\int \frac{d^2p}{p^0} p^\alpha f_{FD}^{eq} = 2\pi\theta^2 g_2(z) U^\alpha = nU^\alpha$ . See below the terms of the expansion.

$$AP = 2A_1^2 g_1(z) \pi\theta, \quad A^{i_1} P^{i_1} = 2B_1^2 (p^x u^x + p^y u^y) g_2(z) \gamma \pi \theta^2$$

$$A^0P^0 = 2\pi\theta(C_2g_1(z) + C_1g_2(z)\gamma\theta)(C_2 + C_1p)$$

$$A^{i_1i_2}P^{i_1i_2} = 2\pi\theta((D_4g_1(z) + \gamma\theta(D_3g_2(z) + g_3(z)\gamma(D_1 + 2D_2 + (2D_1 + D_2)(u^x)^2 + (-D_1 + D_2)(u^y)^2)\theta)) (D_4 + D_3p + D_2p^2 + D_1(p^x)^2) + 6D_1^2g_3(z)\gamma^2u^xu^y\theta^2p^xp^y + (D_4g_1(z) + \gamma\theta(D_3g_2(z) + g_3(z)\gamma(D_1 + 2D_2 +(-D_1 + D_2)(u^x)^2 + (2D_1 + D_2)(u^y)^2)\theta))(D_4 + D_3p + D_2p^2 + D_1(p^y)^2))$$

$$A^{i_10}P^{i_10} = 2(p^xu^x + p^yu^y)\gamma\pi\theta^2(E_2g_2(z) + 3E_1g_3(z)\gamma\theta)(E_2 + E_1p)$$

$$A^{i_1i_2i_3}P^{i_1i_2i_3} = 6\gamma\pi\theta^2(u^x(F_4g_2(z) + \gamma\theta(3F_3g_3(z) + g_4(z)\gamma(F_1(3 + 2(u^x)^2 - 3(u^y)^2) + 3F_2(4 + u^2))\theta)) p^x(3F_4 + 3F_3p + 3F_2p^2 + F_1(p^x)^2) + u^y(F_4g_2(z) + 3\gamma\theta(F_3g_3(z) + g_4(z)\gamma(F_1 + 4F_2 + (4F_1 + F_2)(u^x)^2 +(-F_1 + F_2)(u^y)^2)\theta))(F_4 + F_3p + F_2p^2 + F_1(p^x)^2)p^y + u^x(F_4g_2(z) + 3\gamma\theta(F_3g_3(z) + g_4(z)\gamma(F_1 + 4F_2 +(-F_1 + F_2)(u^x)^2 + (4F_1 + F_2)(u^y)^2)\theta))p^x(F_4 + F_3p + F_2p^2 + F_1(p^y)^2) + u^y(F_4g_2(z) + \gamma\theta(3F_3g_3(z) +g_4(z)\gamma(3F_2(4 + u^2) + F_1(3 - 3(u^x)^2 + 2(u^y)^2))\theta))p^y(3F_4 + 3F_3p + 3F_2p^2 + F_1(p^y)^2))$$

$$A^{i_1i_20}P^{i_1i_20} = 2\pi\theta((g_1(z)G_6 + \gamma\theta(g_2(z)G_5 + \gamma\theta(G_2g_3(z)(1 + 2(u^x)^2 - (u^y)^2) + g_3(z)G_4(2 + u^2) +3g_4(z)\gamma(G_1 + 2G_3 + (4G_1 + 3G_3)(u^x)^2 + (-G_1 + 3G_3)(u^y)^2)\theta)))(G_6 + G_5p + G_4p^2 + G_3p^3 +G_2(p^x)^2 + G_1p(p^x)^2) + 6\gamma^2u^y\theta^2(G_2g_3(z) + 5G_1g_4(z)\gamma\theta)(G_2 + G_1p)p^y((p^xu^x + p^yu^y) - u^yp^y) +(g_1(z)G_6 + g_2(z)G_5\gamma\theta + g_3(z)G_4\gamma^2(2 + u^2)\theta^2 + G_2g_3(z)\gamma^2(1 - (u^x)^2 + 2(u^y)^2)\theta^2 + 3G_3g_4(z)\gamma^3(2 +3u^2)\theta^3 - 3G_1g_4(z)\gamma^3(-1 + (u^x)^2 - 4(u^y)^2)\theta^3)(G_6 + G_5p + G_4p^2 + G_3p^3 + G_2(p^y)^2 + G_1p(p^y)^2))$$

$$A^{i_1i_2i_3i_4}P^{i_1i_2i_3i_4} = 6\pi\theta((g_1(z)H_9 + g_2(z)\gamma H_8\theta + g_3(z)\gamma^2H_7(2 + u^2)\theta^2 + 2g_3(z)\gamma^2H_4(1 + 2(u^x)^2 - (u^y)^2)\theta^2 +3g_4(z)\gamma^3H_6(2 + 3u^2)\theta^3 + 6g_4(z)\gamma^3H_3(1 + 4(u^x)^2 - (u^y)^2)\theta^3 + 3g_5(z)\gamma^4H_5(8 + 24u^2 + 3u^4)\theta^4 + 6g_5(z)\gamma^4H_2 (4 - 3u^2 - u^4 + 5(6 + u^2)(u^x)^2)\theta^4 + g_5(z)\gamma^4H_1(3 + 3u^4 + 30(u^x)^2 + 35(u^x)^4 - 6u^2(1 + 5(u^x)^2))\theta^4)(3(H_9 +p(H_8 + p(H_7 + p(H_6 + H_5p)))) + 6(H_4 + p(H_3 + H_2p))(p^x)^2 + H_1(p^x)^4) + 4\gamma^2u^xu^y\theta^2(3g_3(z)H_4 + 5\gamma\theta (3g_4(z)H_3 + g_5(z)\gamma(H_1(3 + 4(u^x)^2 - 3(u^y)^2) + 3H_2(6 + u^2))\theta))p^x(3H_4 + 3H_3p + 3H_2p^2 + H_1(p^x)^2)p^y +4\gamma^2u^xu^y\theta^2(3g_3(z)H_4 + 5\gamma\theta(3g_4(z)H_3 + g_5(z)\gamma(3H_2(6 + u^2) + H_1(3 - 3(u^x)^2 + 4(u^y)^2))\theta))p^xp^y(3H_4 + 3H_3p +3H_2p^2 + H_1(p^y)^2) + 2(g_1(z)H_9 + \gamma\theta(g_2(z)H_8 + \gamma\theta(g_3(z)(H_4 + H_7)(2 + u^2) + 3\gamma\theta(g_4(z)(H_3 + H_6)(2 +3(u^x)^2 + 3(u^y)^2) - g_5(z)\gamma(-(H_2 + H_5)(8 + 3(u^x)^4 + 24(u^y)^2 + 3(u^y)^4 + 6(u^x)^2(4 + (u^y)^2)) + H_1(-1 +4(u^x)^4 - 3(u^y)^2 + 4(u^y)^4 - 3(u^x)^2(1 + 9(u^y)^2)))\theta))))(H_9 + H_8p + H_7p^2 + H_6p^3 + H_5p^4 + p^2(H_4 + p(H_3 +H_2p)) + H_1(p^x)^2(p^y)^2) + (g_1(z)H_9 + g_2(z)\gamma H_8\theta + g_3(z)\gamma^2H_7(2 + u^2)\theta^2 - 2g_3(z)\gamma^2H_4(-1 + (u^x)^2 -2(u^y)^2)\theta^2 + 3g_4(z)\gamma^3H_6(2 + 3u^2)\theta^3 - 6g_4(z)\gamma^3H_3(-1 + (u^x)^2 - 4(u^y)^2)\theta^3 + 3g_5(z)\gamma^4H_5(8 + 24u^2 + 3u^4)\theta^4 +6g_5(z)\gamma^4H_2(4 - 3u^2 - u^4 + 5(6 + u^2)(u^y)^2)\theta^4 + g_5(z)\gamma^4H_1(3 + 3u^4 + 30(u^y)^2 + 35(u^y)^4 - 6u^2(1 +5(u^y)^2))\theta^4)(3(H_9 + p(H_8 + p(H_7 + p(H_6 + H_5p)))) + 6(H_4 + p(H_3 + H_2p))(p^y)^2 + H_1(p^y)^4))$$

$$A^{i_1i_2i_30}P^{i_1i_2i_30} = 6\gamma\pi\theta^2(u^x(g_2(z)I_6 + \gamma\theta(3g_3(z)I_5 + \gamma\theta(g_4(z)(I_2(3 + 2(u^x)^2 - 3(u^y)^2) + 3I_4(4 + u^2)) +5g_5(z)\gamma(I_1(3 + 4(u^x)^2 - 3(u^y)^2) + 3I_3(4 + 3(u^x)^2 + 3(u^y)^2))\theta)))(3(I_6 + p(I_5 + p\ (I_4 + I_3p)))p^x + (I_2 +I_1p)(p^x)^3) + u^y(g_2(z)I_6 + 3\gamma\theta(g_3(z)I_5 + \gamma\theta(g_4(z)(I_2 + 4I_4 + (4I_2 + I_4)(u^x)^2 + (-I_2 + I_4)(u^y)^2) +5g_5(z)\gamma(I_1 + 4I_3 + 3(2I_1 + I_3)(u^x)^2 + (-I_1 + 3I_3)(u^y)^2)\theta)))(I_6 + I_5p + I_4p^2 + I_3p^3 + (I_2 + I_1p)(p^x)^2)p^y +u^x(g_2(z)I_6 + 3g_3(z)\gamma I_5\theta + 3g_4(z)\gamma^2I_4(4 + u^2)\theta^2 - 3g_4(z)\gamma^2I_2(-1 + (u^x)^2 - 4(u^y)^2)\theta^2 + 15g_5(z)\gamma^3I_3(4 +3u^2)\theta^3 - 15g_5(z)\gamma^3I_1(-1 + (u^x)^2 - 6(u^y)^2)\theta^3)p^x(I_6 + I_5p + I_4p^2 + I_3p^3 + (I_2 + I_1p)(p^y)^2) + u^y(g_2(z)I_6 +\gamma\theta(3g_3(z)I_5 - \gamma\theta(g_4(z)(I_2(-3 + 3(u^x)^2 - 2(u^y)^2) - 3I_4(4 + u^2)) - 5g_5(z)\gamma(3I_3(4 + 3(u^x)^2 + 3(u^y)^2) +I_1(3 - 3(u^x)^2 + 4(u^y)^2))\theta)))(3(I_6 + p(I_5 + p\ (I_4 + I_3p)))p^y + (I_2 + I_1p)(p^y)^3))$$

$$A^{i_1 i_2 i_3 i_4 i_5} P^{i_1 i_2 i_3 i_4 i_5} = 30\gamma\pi\theta^2(u^x(g_2(z)J_9 + g_6(z)\gamma^4 J_1(15\gamma^{-4} - 70(-1+u^2)(u^x)^2 + 63(u^x)^4)\theta^4$$
$$+2\gamma^2\theta^2(g_4(z)J_4(3+2(u^x)^2 - 3(u^y)^2) + 5\gamma\theta(g_5(z)J_3(3+4(u^x)^2 - 3(u^y)^2) + g_6(z)\gamma J_2(4(u^x)^4$$
$$+(u^x)^2(41+(u^y)^2) - 3(-6+5(u^y)^2+(u^y)^4))\theta)) + 3\gamma\theta(g_3(z)J_8 + \gamma\theta(g_4(z)J_7(4+u^2) + 5\gamma\theta$$
$$(g_5(z)J_6(4+3u^2) + 3g_6(z)\gamma J_5(8+12u^2+u^4)\theta))))(15(J_9 + p(J_8 + p(J_7 \ + p(J_6 + J_5 p))))p^x$$
$$+10(J_4 + p(J_3 + J_2 p))(p^x)^3 + J_1(p^x)^5) + u^y(g_2(z)J_9 + 3g_3(z)\gamma J_8\theta + 3g_4(z)\gamma^2 J_7(4+u^2)\theta^2$$
$$+6g_4(z)\gamma^2 J_4(1+4(u^x)^2 - (u^y)^2)\theta^2 + 15g_5(z)\gamma^3 J_6(4+3u^2)\theta^3 + 30g_5(z)\gamma^3 J_3(1+6(u^x)^2$$
$$-(u^y)^2)\theta^3 + 45g_6(z)\gamma^4 J_5(8+12u^2+u^4)\theta^4 + 15g_6(z)\gamma^4 J_1(\gamma^{-4} - 14(-1+u^2)(u^x)^2 + 21(u^x)^4)\theta^4$$
$$-30g_6(z)\gamma^4 J_2(-6+u^4-56(u^x)^2 + u^2(5-7(u^x)^2))\theta^4)(3(J_9 + p(J_8 + p(J_7 + \ p(J_6 + J_5 p))))$$
$$+6(J_4 + p(J_3 + J_2 p))(p^x)^2 + J_1(p^x)^4)p^y + u^x(g_2(z)J_9 + 3g_3(z)\gamma J_8\theta + 3g_4(z)\gamma^2 J_7(4+u^2)\theta^2$$
$$-6g_4(z)\gamma^2 J_4(-1+(u^x)^2 - 4(u^y)^2)\theta^2 + 15g_5(z)\gamma^3 J_6(4+3u^2)\theta^3 - 30g_5(z)\gamma^3 J_3(-1+(u^x)^2$$
$$-6(u^y)^2)\theta^3 + 45g_6(z)\gamma^4 J_5(8+12u^2+u^4)\theta^4 + 15g_6(z)\gamma^4 J_1(\gamma^{-4} - 14(-1+u^2)(u^y)^2$$
$$+21(u^y)^4)\theta^4 - 30g_6(z)\gamma^4 J_2(-6+u^4-56(u^y)^2+u^2(5-7(u^y)^2))\theta^4)p^x(3(J_9 + p(J_8 + p \ (J_7$$
$$+p(J_6 + J_5 p)))) + 6(J_4 + p(J_3 + J_2 p))(p^y)^2 + J_1(p^y)^4) + 2u^x(g_2(z)J_9 + \gamma\theta(3g_3(z)J_8 + \gamma\theta(g_4(z)$$
$$(3J_7(4+u^2) + J_4(6-(u^x)^2 + 9(u^y)^2)) + 5\gamma\theta(g_5(z)(3J_6(4+3(u^x)^2+3(u^y)^2) + J_3(6+(u^x)^2$$
$$+15(u^y)^2)) - g_6(z)\gamma(-9J_5(8+(u^x)^4 + 12(u^y)^2 + (u^y)^4 + 2(u^x)^2(6+(u^y)^2)) - J_2((u^x)^4$$
$$+2(u^x)^2(13+8(u^y)^2) + 3(12+46(u^y)^2+5(u^y)^4)) + J_1(4(u^x)^4 - (u^x)^2(1+41(u^y)^2) + 3(-1$$
$$-5(u^y)^2 + 6(u^y)^4)))\theta))))p^x(3J_9 + 3J_8 p + (J_4 + 3J_7)(p^x)^2 + (J_3 + 3J_6)p(p^x)^2 + (J_2 + 3J_5)(p^x)^4$$
$$+3(J_4 + J_7)(p^y)^2 + 3(J_3 + J_6)p(p^y)^2 + (J_1 + 4J_2 + 6J_5)(p^x)^2(p^y)^2 + 3(J_2 + J_5)(p^y)^4)$$
$$+2u^y(g_2(z)J_9 + \gamma\theta(3g_3(z)J_8 + \gamma\theta(g_4(z)(J_4(6+9(u^x)^2 - (u^y)^2) + 3J_7(4+u^2)) + 5\gamma\theta(g_5(z)$$
$$(J_3(6+15u^2) + 3J_6(4+3(u^x)^2+3(u^y)^2)) - g_6(z)\gamma(-9J_5(8+(u^x)^4+12(u^y)^2+(u^y)^4$$
$$+2(u^x)^2(6+(u^y)^2)) - J_2(36+15(u^x)^4+26(u^y)^2+(u^y)^4+2(u^x)^2(69+8(u^y)^2)) + J_1(-3$$
$$+18(u^x)^4 - (u^y)^2 + 4(u^y)^4 - (u^x)^2(15+41(u^y)^2)))\theta))))p^y(3J_9 + 3J_8 p + 3(J_4 + J_7)(p^x)^2$$
$$+3(J_3 + J_6)p(p^x)^2 + 3(J_2 + J_5)(p^x)^4 + (J_4 + 3J_7)(p^y)^2 + (J_3 + 3J_6)p(p^y)^2 + (J_1 + 4J_2$$
$$+6J_5)(p^x)^2(p^y)^2 + (J_2 + 3J_5)(p^y)^4) + u^y(g_2(z)J_9 + g_6(z)\gamma^4 J_1(15\gamma^{-4} - 70(-1+u^2)(u^y)^2$$
$$+63(u^y)^4)\theta^4 + 2\gamma^2\theta^2(g_4(z)J_4(3-3(u^x)^2+2(u^y)^2) + 5g_5(z)\gamma J_3(3-3(u^x)^2+4(u^y)^2)\theta$$
$$+5g_6(z)\gamma^2 J_2(18-3u^4+56(u^y)^2+u^2(-15+7(u^y)^2))\theta^2) + 3\gamma\theta(g_3(z)J_8 + \gamma\theta(g_4(z)J_7(4$$
$$+u^2) + 5\gamma\theta(g_5(z)J_6(4+3u^2) + 3g_6(z)\gamma J_5(8+12u^2+u^4)\theta))))(15(J_9 + p(J_8 + p(J_7 \ + p(J_6$$
$$+J_5 p))))p^y + 10(J_4 + p(J_3 + J_2 p))(p^y)^3 + J_1(p^y)^5))$$

$$A^{i_1 i_2 i_3 i_4 0} P^{i_1 i_2 i_3 i_4 0} = 6\pi\theta((g_1(z)K_{12} + g_2(z)\gamma K_{11}\theta + g_3(z)\gamma^2 K_{10}(2+u^2)\theta^2 + 2g_3(z)\gamma^2 K_6(1+2(u^x)^2 -(u^y)^2)\theta^2 + 3g_4(z)\gamma^3 K_9(2+3u^2)\theta^3 + 6g_4(z)\gamma^3 K_5(1+4(u^x)^2 - (u^y)^2)\theta^3 + 3g_5(z)\gamma^4 K_8(8+24u^2 +3u^4)\theta^4 + 6g_5(z)\gamma^4 K_4(4-3u^2-u^4+5(6+u^2)(u^x)^2)\theta^4 + g_5(z)\gamma^4 K_2(3+3u^4+30(u^x)^2+35(u^x)^4 -6u^2(1+5(u^x)^2))\theta^4 + 15g_6(z)\gamma^5 K_7(8+40u^2+15u^4)\theta^5 + 15g_6(z)\gamma^5 K_1(\gamma^{-4} - 14(-1+u^2)(u^x)^2 +21(u^x)^4)\theta^5 - 30g_6(z)\gamma^5 K_3(-4+3u^4-42(u^x)^2+u^2(1-21(u^x)^2))\theta^5)(3(K_{12}+p(K_{11}+p(K_{10} +p(K_9+p(K_8+K_7p))))) + 6(K_6+p(K_5+p(K_4+K_3p)))(p^x)^2 + (K_2+K_1p)(p^x)^4) + 6\gamma^2 u^x u^y \theta^2 (3g_3(z)K_6 + 5\gamma\theta(3g_4(z)K_5 + \gamma\theta(g_5(z)(K_2(3+4(u^x)^2-3(u^y)^2) + 3K_4(6+u^2)) + 21g_6(z)\gamma(K_1(1 +2(u^x)^2-(u^y)^2) + 3K_3(2+(u^x)^2+(u^y)^2))\theta))) \cdot (3(K_6+p(K_5+p(K_4+K_3p)))p^x p^y + (K_2 +K_1p)(p^x)^3 p^y) + 2(g_1(z)K_{12} + \gamma\theta(g_2(z)K_{11} + \gamma\theta(g_3(z)(K_{10}+K_6)(2+u^2) + 3\gamma\theta(g_4(z)(K_5+K_9) (2+3(u^x)^2+3(u^y)^2) + \gamma\theta(g_5(z)((K_4+K_8)\cdot(8+24u^2+3u^4) + K_2(1+3u^2-4u^4+35(u^x)^2(u^y)^2)) +5g_6(z)\gamma((K_3+K_7)(8+40u^2+15u^4) + K_1(1+5u^2-6u^4+63(u^x)^2(u^y)^2))\theta)))))(K_{12}+K_{11}p +K_{10}p^2+K_9p^3+K_8p^4+K_7p^5+p^2(K_6+p(K_5+p(K_4+K_3p))) + (K_2+K_1p)(p^x)^2(p^y)^2) +4\gamma^2 u^x u^y \theta^2(3g_3(z)K_6 + 5\gamma\theta(3g_4(z)K_5 - \gamma\theta(g_5(z)(K_2(-3+3(u^x)^2-4(u^y)^2) - 3K_4(6+u^2)) -21g_6(z)\gamma(3K_3(2+u^2) + K_1(1-(u^x)^2+2(u^y)^2))\theta)))(3(K_6+p(K_5+p\ (K_4+K_3p)))p^x p^y + (K_2 +K_1p)p^x(p^y)^3) + (g_1(z)K_{12} + g_2(z)\gamma K_{11}\theta + g_3(z)\gamma^2 K_{10}(2+u^2)\theta^2 - 2g_3(z)\gamma^2 K_6(-1+(u^x)^2 -2(u^y)^2)\theta^2 + 3g_4(z)\gamma^3 K_9(2+3u^2)\theta^3 - 6g_4(z)\gamma^3 K_5(-1+(u^x)^2-4(u^y)^2)\theta^3 + 3g_5(z)\gamma^4 K_8(8+24u^2 +3u^4)\theta^4 + 6g_5(z)\gamma^4 K_4(4-3u^2-u^4+5(6+u^2)(u^y)^2)\theta^4 + g_5(z)\gamma^4 K_2(3+3u^4+30(u^y)^2+35(u^y)^4 -6u^2(1+5(u^y)^2))\theta^4 + 15g_6(z)\gamma^5 K_7(8+40u^2+15u^4)\theta^5 + 15g_6(z)\gamma^5 K_1(\gamma^{-4} - 14(-1+u^2)(u^y)^2 +21(u^y)^4)\theta^5 - 30g_6(z)\gamma^5 K_3(-4+3u^4-42(u^y)^2+u^2(1-21(u^y)^2))\theta^5)(3(K_{12}+p(K_{11}+p(K_{10} +p(K_9+p(K_8+K_7p))))) + 6(K_6+p(K_5+p(K_4+K_3p)))(p^y)^2 + (K_2+K_1p)(p^y)^4))$$

For a discrete version of this distribution function, it is enough to change the momentum vectors by the discrete ones given in section II, $p^\alpha \to p_i^\alpha$, and do the same for the weight function, $\omega(p) \to w_i$. We used constant Fermi-Dirac integrals $g_\nu(z)$, since $\mu = 0 \to z = 1$, but it could be straightforwardly generalized for other chemical potentials. See bellow the values we used:

| Fermi-Dirac integrals for $\mu = 0$ | |
|---|---|
| $g_1(1)$ | 0.69314718055994530942 |
| $g_2(1)$ | 0.82246703342411321824 |
| $g_3(1)$ | 0.90154267736969571405 |
| $g_4(1)$ | 0.94703282949724591758 |
| $g_5(1)$ | 0.97211977044690930594 |
| $g_6(1)$ | 0.98555109129743510409 |


[1] M. Mendoza, B. M. Boghosian, H. J. Herrmann, and S. Succi, Phys. Rev. Lett. **105**, 014502 (2010).

[2] T. Krüger, H. Kusumaatmaja, A. Kuzmin, O. Shardt, G. Silva, and E. Viggen, *The Lattice Boltzmann Method: Principles and Practice*, Graduate Texts in Physics (Springer International Publishing, 2016).

[3] M. Müller, J. Schmalian, and L. Fritz, Phys. Rev. Lett. **103**, 025301 (2009).

[4] R. C. V. Coelho, A. Ilha, M. M. Doria, R. M. Pereira, and V. Y. Aibe, Phys. Rev. E **89**, 043302 (2014).

[5] M. M. Doria and R. C. V. Coelho, ArXiv e-prints (2017), arXiv:1703.08670 [math-ph].

[6] R. C. V. Coelho, A. S. Ilha, and M. M. Doria, EPL (Europhysics Letters) **116**, 20001 (2016).

[7] C. Cercignani and G. M. Kremer, "Relativistic boltzmann equation," in *The Relativistic Boltzmann Equation: Theory and Applications* (Birkhäuser Basel, Basel, 2002).
